# Supplementary material for: Wireless-Powered Two-Way Relaying with Power Splitting-based Energy Accumulation
Source: arXiv:1608.01859 source file (2016-08-05)
Supplement: Supplementary file 1 [file Appendix_A.tex]

\subsection{Proof of Lemma \ref{lemma:PDF}}\label{append:proof_lemma_PDF}
